# Supplementary material for: Prompt-responsive Object Retrieval with Memory-augmented Student-Teacher Learning
Source: arXiv:2505.02232 source file (2025-05-04)
Supplement: Supplementary file 1 [file appendix.tex]

\begin{appendices}
    \setcounter{figure}{0}
    \setcounter{table}{0}
    \setcounter{footnote}{0}

    \section{Sim-to-Real Transfer}

    \subsection{Hand Dynamics Identification}
    \label{sec:hand_dynamics_identification}
    The Schunk SIH hand used in this work is a tendon-driven system with 5 actuators and 11 degrees of freedom. 
    Closing the hand by actuating the motors results in complex joint-angle responses that are difficult to replicate in simulation. 
    Further, the hand is not equipped with joint encoders, making it difficult to obtain ground truth joint angles during deployment or for calibration.

    The bump on the index finger calibration line is caused by the collision with the thumb inter pad and does not need to be modelled. Instead, remove the thumb during calibration.

    \begin{figure*}[t]
        \centering
        \includegraphics[width=\textwidth]{figures/sih_calibration.pdf}
        \caption{Test caption.}
        \label{fig:sih_calibration}
    \end{figure*}

    \section{Experimental Setup}
    The used robot combines a Universal Robot UR5 arm and Schunk SIH hand.

    \section{Policy Interface}

\end{appendices}
